# Supplementary material for: Controlling Repetition in Protein Language Models
Source: arXiv:2602.00782 source file (2026-01-31)
Supplement: Supplementary file 1 [file appendix_case_examples.tex]

\setlength{\tabcolsep}{3pt}

% Column types for xltabular
\newcolumntype{L}{>{\RaggedRight\arraybackslash}p{0.10\textwidth}}
\newcolumntype{I}{>{\RaggedRight\arraybackslash}p{0.18\textwidth}}
\newcolumntype{Xtt}{>{\ttfamily\footnotesize\RaggedRight\arraybackslash}X}
\newcolumntype{C}{>{\centering\arraybackslash}p{0.06\textwidth}}
\begin{xltabular}{\textwidth}{L I Xtt C C C C C}
\caption{Sequence-level metrics for representative examples used in Figure~\ref{fig:case_panel}. Lower values on repetition metrics indicate more repetition.}\label{tab:case-metrics}\\
\toprule
Dataset & Seq ID & \texttt{Sequence} & $H_{\mathrm{norm}}$ & $\mathrm{Distinct}\!-\!n$ & $R_{\mathrm{hpoly}}$ & $\mathrm{pLDDT}$ & $\mathrm{pTM}$ \\
\midrule
\endfirsthead
\multicolumn{8}{l}{\emph{(continued)}}\\
\toprule
Dataset & Seq ID & \texttt{Sequence} & $H_{\mathrm{norm}}$ & $\mathrm{Distinct}\!-\!n$ & $R_{\mathrm{hpoly}}$ & $\mathrm{pLDDT}$ & $\mathrm{pTM}$ \\
\midrule
\endhead
CATH & cath|4\_4\_0|5ty0A02/292-404 & \seqsplit{DIQGVDEHGDVIHRKTSYDEPFSALAFKIATDPFVGTLTYFRAYSGILKSGDTVYNSVKGKKERIGRLLQMHANSREEIKEVRAGDIAAAVGLKTVTTGDTLCDQDKVVILERMDFPDPVIAVAVEPK} & 0.932 & 0.890 & 1.000 & 0.975 & 0.874 \\
ESM3 & esm3\_gen\_seq\_008002 & \seqsplit{MRSSSSSSALLLLLLLLLLLFLLFLLFLLLLLLLLLSSESSSLSSSSSSRSSSSSSSSINASSSSSSSSHSSSSSSSSSSSSSSSSSSSSASRSSSSSSSSNSSSPLSSSSSSSSSPPLLLLSFST} & 0.428 & 0.273 & 0.294 & 0.622 & 0.363 \\
SCOP & 8059848 & \seqsplit{TPTFLVCPDVVKFENVGQIAVVNGMVYLGGSVGIDKSGTLHKGLEEQTRQTFDNIRKCLEYANSGLDYIVSLNIFLSTSLSDSEEARFNELYREVFCVPATRPCRCCVRAQLQEGLLVEVVNVVAAQK} & 0.934 & 0.909 & 1.000 & 0.987 & 0.938 \\
UNITPROT & sp|Q8DQS7|MRNC\_STRR6 & \seqsplit{MIDVNLINGIALAFEGDAVYSMYIRRHLILKGMTKPNKLHQEATKYVSAKAQARLIALMLEEQVLTEKEEEIYKRGRNTNSHTKAKNADVVTYRMSTGFEAVMGYLHMTENLERLESLVSWCIQKVEG} & 0.939 & 0.905 & 1.000 & 0.987 & 0.932 \\
CATH & cath|4\_4\_0|2dcmA02/477-732 & \seqsplit{AMPEIRTGTIMAADGQTPLYYKLTMPLHFDPAKKYPVIVYVYGGPHAQLVTKTWRSSVGGWDIYMAQKGYAVFTVDSRGSANRGAAFEQVIHRRLGQTEMADQMCGVDFLKSQSWVDADRIGVHGWAYGGFMTTNLMLTHGDVFKVGVAGGPVIDWNRYEIMYGERYFDAPQENPEGYDAANLLKRAGDLKGRLMLIHGAIDPVVVWQHSLLFLDACVKARTYPDYYVYPSHEHNVMGPDRVHLYETITRYFTDHL} & 0.964 & 0.835 & 1.000 & 0.973 & 0.952 \\
ESM3 & esm3\_gen\_seq\_009137 & \seqsplit{AAAAAAALAALAASNAAAGAAAAAAAAAAAAARAAAAAADLLAVALAAVAAFAAAAAAAAGAAAAAAAAKKLAAAARAAAAAAAAAAAAAAAAIAAAFEAAAAGAAVAAAAAAAAAGAAAAAAAADAAAAAAAAAAAAARLANAAAAAAAALGAAAAAAAAGAAAAASAAALAQNGGAAAAAAAAAAAAAAAAAVAAAGAAAAAAAAAARAAAALAAAAAALAAAAAALAEAAGAAAAAAPIAARSFLAAALAQAA} & 0.327 & 0.200 & 0.352 & 0.686 & 0.675 \\
SCOP & 8068106 & \seqsplit{KRLEGKSALITGSARGIGRAFAEAYVREGATVAIADIDIERARQAAAEIGPAAYAVQMDVTRQDSIDAAIAATVEHAGGLDILVNNAALFDLAPIVEITRESYEKLFAINVAGTLFTLQAAARQMIAQGRGGKIINMASQAGRRGEALVAIYCATKAAVISLTQSAGLDLIKHRINVNAIAPGVVDGEHWDGVDALFARYENRPRGEKKRLVGEAVPFGRMGTAEDLTGMAIFLASAESDYIVSQTYNVDGGNWMS} & 0.911 & 0.757 & 1.000 & 0.983 & 0.955 \\
UNITPROT & sp|Q8XGF9|GARL\_SALTI & \seqsplit{MNNAIFPNKFKAALAAQQVQIGCWSALASPITTEVLGLAGFDWLVLDGEHAPNDVTTLIPQLMALKGSASAPVVRVPTNEPVIIKRMLDIGFYNFLIPFVETQEEAARAVASTRYPPEGIRGVSVSHRANMFGTVPDYFAQSNKNITIIVQIESQLGVDNVDAIAATEGVDGIFVGPSDLAAALGHLGNASHPDVQQTIQHIFARAKAHGKPCGILAPVEADARRYLEWGATFVAVGSDLGAFRASTQKLADTFKK} & 0.941 & 0.806 & 1.000 & 0.985 & 0.941 \\
CATH & cath|4\_4\_0|5ewqC00/32-536 & \seqsplit{SNAYKNYFPKEPERIVYDKERVLQPIHNQLKGINIENVKIKEKEVVNATVDELQKMIDDGKLSYEELTSIYLFRIQEHDQNGITLNSVTEINPNAMEEARKLDQERSRNKKSNLYGIPVVVKDNVQTAKVMPTSAGTYVLKDWIADQDATIVKQLKEEGAFVLGKANMSEWANYLSFTMPSGYSGKKGQNLNPYGPIMFDTSGSSSGSATVVAADFAPLAVGTETTGSIVAPAAQQSVVGLRPSLGRVSRTGIIPLAETLDTAGPMARTVKDAATLFNAMIGYDEKDVMTEKVKDKERIDYTKDLSIDGLKGKKIGLLFSVDQQDENRKAVAEKIRKDLQDAGAILTDYIQLNNGGVDNLQTLEYEFKHNVNDYFSQQKNVPVKSLKEIIAFNKRDSNRRIKYGQTLIEASEKSTITKDEFEKVVQTSQENAKKELNKYLVEKGLDALVMINNEEVLLSAVAGYPELAVPAGYDNNGEPVGAVFVGKQFGEKELFNIGYAYEQQSKNRKPPKL} & 0.935 & 0.693 & 1.000 & 0.933 & 0.932 \\
ESM3 & esm3\_gen\_seq\_003255 & \seqsplit{MLILLLLLLLLLLYLLLLLILLLLLLLSLLLLLLILLLLLFLFSFSLLLSLSILLLLLLLLLLLLLLLLLLGLALLLLLKLLLLLLLLLLLLLLLLLLLLLLLLLVLLLLLLLLLLPLLLLLLLLGLAVLLLILLLLLLLLLILSLLSFSLLLLKLALLLLLLLLLLLLLLLLLLLLLLLLLLLLLLLLLLLLALLLLLLGLLLLGLLSLLLSLLLLLLLLALLALLLLLLFLLLQLLLLLLLLPLLLLLLLLLLLLLLGLLLILLILLLALLFLLLLLVSLLLLELLLLLPALLYALLLLLLRLLLLLLLLLLPVLLLLLLLLLLLLLLLFLLLLLLLLLLLLLLKLLILLLLLLLLLLLVAALLLLLSLGLLLLLFLLLLGNLLLLLLLLLLFSLLLLLILLLLLLLFLLLSISLLILSLLLLLLCSLLLLLLSSLLSLLLVEKLSLLLLLSLLLLLLLLLLHLLLMLLLLLLLLLLLLVLFLGLFLLLLLALLLLLPLLLSLLLLLLLL} & 0.301 & 0.131 & 0.303 & 0.569 & 0.204 \\
SCOP & 8022308 & \seqsplit{HKHAIPANIADRCLINPEQYETKYKQSINDPDTFWGEQGKILDWITPYQKVKNTSFAPGNVSIKWYEDGTLNLAANCLDRHLQENGDRTAIIWEGDDTSQSKHISYRELHRDVCRFANTLLDLGIKKGDVVAIYMPMVPEAAVAMLACARIGAVHSVIFGGFSPEAVAGRIIDSSSRLVITADEGVRAGRSIPLKKNVDDALKNPNVTSVEHVIVLKRTGSDIDWQEGRDLWWRDLIEKASPEHQPEAMNAEDPLFILYTSGSTGKPKGVLHTTGGYLVYAATTFKYVFDYHPGDIYWCTADVGWVTGHSYLLYGPLACGATTLMFEGVPNWPTPARMCQVVDKHQVNILYTAPTAIRALMAEGDKAIEGTDRSSLRILGSVGEPINPEAWEWYWKKIGKEKCPVVDTWWQTETGGFMITPLPGAIELKAGSATRPFFGVQPALVDNEGHPQEGATEGNLVITDSWPGQARTLFGDHERFEQTYFSTFKNMYFSGDGARRDEDGYYWITGRV} & 0.971 & 0.728 & 1.000 & 0.961 & 0.948 \\
UNITPROT & sp|A5CD07|ATPA\_ORITB & \seqsplit{MQLKASEVYEALKQQLEDFDELSELSEVGYVISIGDGIAKVYGLSNAYSGEILQFSTGTKGIVFSLKDNLIEVVVIGSGDQIKQGSQVKRTQTSLKVPTGKELLGRVVDAIGNPIDGKGEFINPTYLDVEVKAPSVMCRDSVNEPMYTGIKAIDALIPIGKGQRELIIGDRQTGKTAIAIDIILNQKRFHLSDQEKEKVYCIYVAIGQKRSTVAQLVKKLQETGAMAYTTVVLSSASDAASLQYLAPYTGCAIGEYFRDNCMHALVIYDDLSKHAIAYRQISLLLRRPPAREAYPGDVFYLHSRLLERAAKLNKAKGEGSLTALPIVETQNSDVSAYIPTNIISITDGQIFLESELFYKGIKPALNVGISVSRVGAAAQIKAMKDIASSVKLELAQYHEMEAFSQFGADLDSSSMQLINRGRRLSELLKQSQYCPFPVEEQIIVLFAGINGYLDKIAVSKVKEFENNMLEYFRIHNPDIMNEIINTKKITEIISSKLHQILQEFVKSIEQCS} & 0.940 & 0.704 & 1.000 & 0.983 & 0.948 \\
\bottomrule
\end{xltabular}
