# Supplementary material for: Controlling Repetition in Protein Language Models
Source: arXiv:2602.00782 source file (2026-01-31)
Supplement: Supplementary file 2 [file appendix_example.tex]

\begin{table}
\centering
\caption{Sequence-level metrics for representative examples used in Figure~\ref{fig:case_panel}. Lower values on repetition metrics indicate more repetition.}\label{tab:case-metrics}
\resizebox{0.9\linewidth}{!}{
\begin{tabular}{ccccccc}
\toprule
\texttt{Sequence} & \multicolumn{6}{c}{MRSSSSSSALLL LLLLLLLLFLLF LLFLLLLLLLLL SSESSSLSSSSSS RSSSSSSSSINAS SSSSSSSHSSSSS SSSSSSSSSSSSS SSASRSSSSSSSS NSSSPLSSSSSSS SSPPLLLLSFST} \\
Dataset & Seq ID & $H_{\mathrm{norm}}$ & $\mathrm{Distinct}\!-\!n$ & $R_{\mathrm{hpoly}}$ & $\mathrm{pLDDT}$ & $\mathrm{pTM}$\\
\bottomrule
\end{tabular}
}
\end{table}
